# Supplementary material for: Enhancing reactivity of SiO$^+$ ions by controlled excitation to extreme rotational states
Source: arXiv:2209.09129 ancillary file (2025-01-11)
Supplement: Supplementary file 1 [file SI.pdf]

## Supporting Information

# Rotational control of reactivity: Reaction of $\text{SiO}^+$ ions in extreme rotational states

Sruthi Venkataramanababu<sup>1,2</sup>, Anyang Li<sup>3,\*</sup>, Ivan Antonov<sup>4</sup>, James Dragan<sup>2</sup>,  
Patrick Stollenwerk<sup>5</sup>, Hua Guo<sup>6</sup> and Brian Odom<sup>2,\*</sup>

<sup>1</sup>Applied Physics Program, Northwestern University, Evanston, 60201, IL, USA

<sup>2</sup>Department of Physics, Northwestern University, Evanston, 60201, IL, USA

<sup>3</sup>Key Laboratory of Synthetic and Natural Functional Molecule Chemistry, Ministry of Education, College of Chemistry and Materials Science, Northwest University, 710127 Xi'an, P. R. China

<sup>4</sup>Lebedev Physical Institute, Samara, 443011, Russian Federation

<sup>5</sup>Argonne National Laboratory, Lemont, 60439, IL, USA

<sup>6</sup>Department of Chemistry and Chemical Biology, University of New Mexico, Albuquerque, 87131, New Mexico, USA

## I. Trapping, optical pumping, and in-situ mass spectrometry

Experiments to measure the reaction rate are conducted in an ion trap where  $\text{SiO}^+$  ions are co-loaded with  $\text{Ba}^+$  ions. The  $\text{SiO}^+$  ions are optically pumped into desired rotational states using a broadband optical pumping method. The techniques for ion trapping, in-situ mass spectrometry and optical pumping are described in Fig. S1

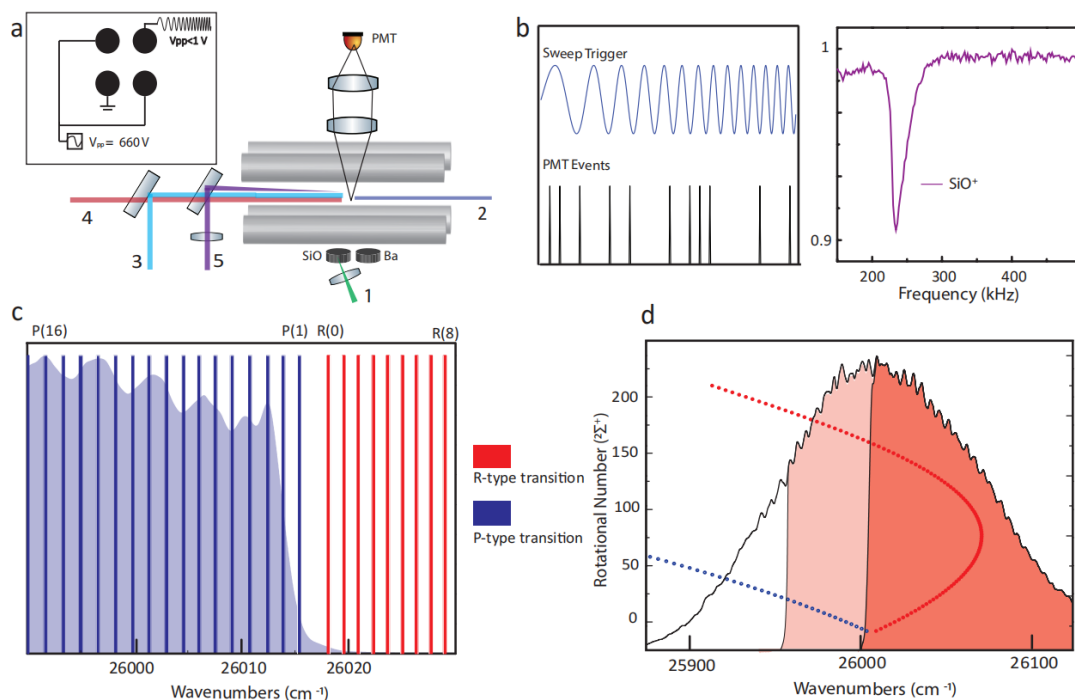

**Fig. S1 a:** The experimental setup consists of a linear ion trap, into which  $\text{Ba}^+$  and  $\text{SiO}^+$  ions are loaded via ablation (1) followed by photoionization (2). The  $\text{Ba}^+$  ions are Doppler cooled continuously using the 493 nm (3) and 650 nm lasers (4). The  $\text{Ba}^+$  cloud cools the translational motion of  $\text{SiO}^+$ . Rotational control is achieved via a broadband laser centered at 385 nm (5). Inset shows a top-view of the trap with the RF voltages and low-voltage chimp that is applied to the rods. **b: Left:** The waveform of the low-voltage chimp that is applied to the trap rods and the PMT events as a result of the low-voltage excitation. **Right:** When the chimp frequency resonates with the  $\text{SiO}^+$  motion, the fluorescence of  $\text{Ba}^+$  goes down; we monitor the center frequency of the dip in fluorescence and use that for in-situ mass spectrometry. **c:** Spectral mask used to pump  $\text{SiO}^+$  to  $j=1/2$ . Blue (Red) sticks represent the P (R) branch, shaded region represents the intensity of light. To pump into  $j=1/2$ , all R branch transitions are blocked, allowing only P-type transitions. **d:** In step 1, (dark red), the spectral mask pumps  $\text{SiO}^+$  to around  $j=170$  (super-rotors) by allowing only R-type transitions and completely blocking out all P-type transitions. In step 2 (light red), we expose an additional section of the spectra corresponding to R-type transitions to take the molecule to even higher rotational states ( $j=170$  and onwards).

## II. SiO<sup>+</sup> population distribution calculations via Einstein rate equations

Spectra of the X-X, X-A, X-B and A-B systems were simulated with the PGOPHER package using ab initio calculations and experimental data from.<sup>1</sup> Permanent electric dipole and transition dipole curves for the X, A, and B states were obtained from ab initio calculations.<sup>2,3</sup> Deperturbed vibrational constants were used in RKR inversion to reconstruct the potential energy curves of the X, A, and B states. The number of vibronic levels for RKR was limited to 3, i.e.  $v = 0 - 2$  for all electronic states. Each vibrational level included rotational states  $j = 0.5 - 199.5$ . Optical pumping, radiative relaxation and interactions with blackbody radiation were then simulated by numerically solving a set of first-order rate equations for all 4800 states included in the simulation. Further details regarding the simulations can be found in the work by *J.Dragan et.al* (<https://arxiv.org/abs/2208.14296>).

The population time evolution for  $t = 0 - 100$  s is calculated starting from the initial state vector in which the population is equally distributed between  $j = 13.5$  and  $j=15.5$  of the  $X, v=0$  level. The population evolution is largely complete at  $t = \sim 1$ s. Fig. S2 shows fractional populations in rotational levels of  $X, v=0$  and  $A, v=0$  states at  $t=100$  s. The selected vibronic levels account for 91.6% of total population with most of it being in the  $A, v=0$  state which becomes the ground vibronic state at high  $j$ . The remaining 8.4% of population is mostly located in the  $A, v=1$  state. The mechanism of populating the high  $j$  levels in the X and A states is the following: pumping the highly diagonal X-B transition followed by radiative decay of the B state results in a quick increase of the rotational quantum number of the X state. Near  $j = 145.5$ ,  $A, v=0$  state becomes lower in energy than  $X, v=0$ ; however, the latter is sufficiently metastable to continue increase in  $j$  via the X-B transition pumping. The population of the A state slowly accumulates via the X-A and B-A radiative decay processes. The complex shape of population curves vs  $j$  in  $X, v=0$  and  $A, v=0$  is determined by perturbation between selected rotational levels of  $X, v=0$  and  $A, v=0,1$  states which occur near  $j = 140$  and  $165$ . The perturbation results in increased probability of radiative decay and pumping via the B-A transition due to intensity borrowing from B-X. The population in the excited rotational levels

of the  $A, v=0$  state slowly decays radiatively down the rotational level ladder until it reaches  $j = 145.5$  at which point it may go back to  $X, v=0$  state and undergo rotational pumping via  $X$ - $B$  transition by the laser field. Alternatively, it may undergo direct  $A$ - $B$  excitation after which the molecule in the  $B$  state preferentially decays to  $X$  state and undergoes  $X$ - $B$  excitation.

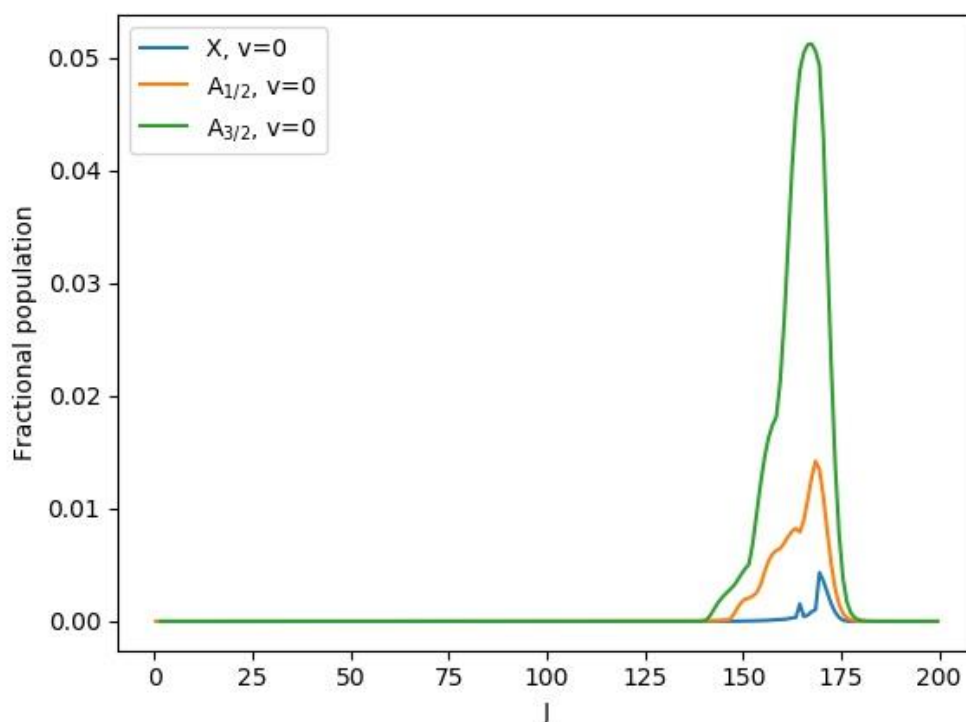

**Fig. S2** Rotational populations of  $\text{SiO}^+$  in  $X, v=0$  and  $A, v=0$  after 100 seconds of optical pumping.

### III. Gaussian Decomposition

The LCFMS mass spectrum has a  $m/\Delta m$  of  $\sim 30$  and thus it cannot resolve the  $\text{SiO}^+$  and  $\text{SiOH}^+$  peaks. However, the mass spectrum can be fitted to a sum of two Gaussians centered at two different frequencies corresponding to the secular frequencies of  $\text{SiO}^+$  and  $\text{SiOH}^+$ . As the  $\text{SiO}^+$  reacts to form  $\text{SiOH}^+$ , the amplitude of the  $\text{SiO}^+$  Gaussian drops while that of the  $\text{SiOH}^+$  Gaussian rises. Consequently, the effective Gaussian shifts towards lower frequencies as the reaction proceeds indicating an increase in the  $\text{SiOH}^+$  concentration in the trap.

Mathematically, by writing a Gaussian function in a Taylor's series expansion, it is possible to show that,

$$G(x-x_{0,3}) = a \cdot G(x-x_{0,1}) + (1-a) \cdot G(x-x_{0,2}), \quad (i)$$

where  $G(x-x_{0,i})$  is a Gaussian centered around  $x_{0,i}$ . The two Gaussians centered around  $x_{0,1}$  and  $x_{0,2}$  are assumed to have the same width.

here  $x_{0,3} = (x_{0,1}-x_{0,2}) \cdot a + x_{0,2}$ , here  $x_{0,3}$ ,  $x_{0,2}$  and  $x_{0,1}$  are the centers of the effective Gaussian, Gaussian centered at  $\text{SiO}^+$  and Gaussian centered at  $\text{SiOH}^+$  respectively, and  $a$  is the amplitude of the Gaussian centered at  $\text{SiO}^+$ .

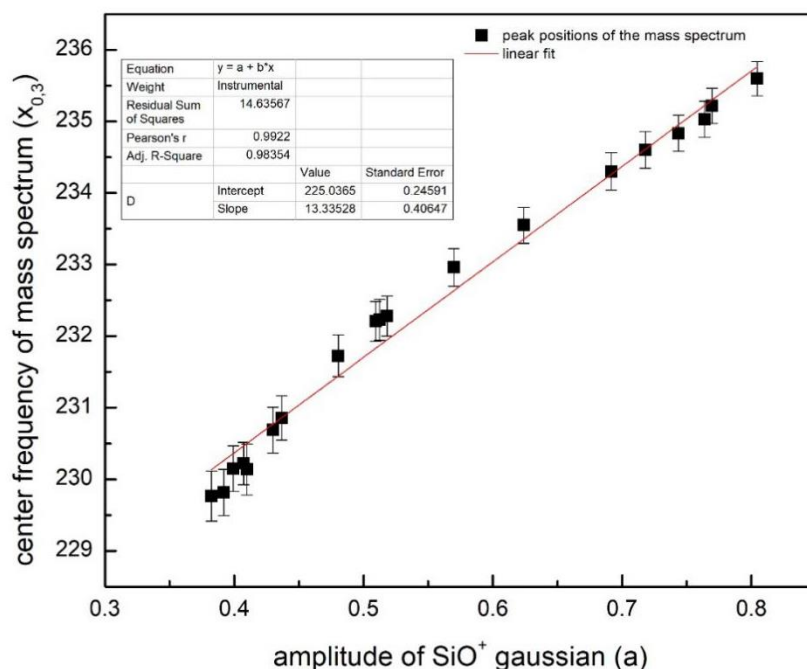

**Fig. S3** Linearity between the amplitude of  $\text{SiO}^+$  and the position of the peak of the mass spectrum

## IV. Singular Value Decomposition

As  $\text{SiO}^+$  reacts away to form  $\text{SiOH}^+$ , the dip in fluorescence shifts to lower frequencies, reflecting an increase in  $\text{SiOH}^+$  concentration. The resolving power of the LCFMS technique in our ion trap is  $m/\Delta m = 30$  and thus it cannot resolve between  $\text{SiO}^+$  (mass 44) and  $\text{SiOH}^+$  (mass 45). Moreover, the fluorescence of  $\text{Ba}^+$  fluctuates due to drifts in frequency, on the order of

a few MHz, of the lasers used to Doppler-cool Ba<sup>+</sup>. On rare occasions, this also led to a loss of SiO<sup>+</sup> ions from the trap if the drift was larger than 5 MHz. To deal with the noise from fluorescence fluctuations, we used singular value decomposition (SVD) of the data to effectively isolate amplitude variations in fluorescence and mass-dependent frequency shift of the fluorescence spectrum. With sufficient averaging, and by appropriately employing SVD analysis, we inferred the rate of reaction of SiO<sup>+</sup>.

The 2-D matrix (**R**) in Fig.S4a is the experimental data; it represents the depletion in Ba<sup>+</sup> fluorescence as function of the chirp frequency and time. **R** has dimensions **m x n**, **m** for chirp frequency and **n** for time. SVD factorizes **R** such that **R = U Σ V\*** where **U** has the dimensions of **m x m** and **V** has dimensions of **n x n** and **U** and **V** are unitary matrices. **Σ** is a diagonal **m x n** matrix with the diagonal entries being ordered from the largest to smallest values. SVD of any matrix can be used to obtain a weighted and ordered sum of several constituent matrices. We now rewrite **R** as **R = Σ<sub>i</sub> σ<sub>i</sub> U<sub>i</sub> V<sub>i</sub>**, where **σ<sub>i</sub>** are the ordered values from the diagonal of **Σ** and **U<sub>i</sub>** and **V<sub>i</sub>** are *i*<sup>th</sup> columns of **U** and **V\*** respectively. **σ<sub>i</sub>**'s weigh the contribution of each of the separable matrices **U<sub>i</sub> V<sub>i</sub>** to the original matrix. Writing the original matrix in terms of its SVD decomposition reveals characteristic patterns in data that may otherwise not be noticeable due to noise and size of the data. In our case, we would like to understand the kinetics of SiOH<sup>+</sup> production and the consequent shift in the fluorescence spectrum to lower frequencies by isolating it from the intensity and linewidth fluctuations in fluorescence. The first few values of **σ<sub>i</sub>** are of appreciable intensity, the rest are very small positive numbers indicating that the first few elements of **Σ<sub>i</sub> σ<sub>i</sub> U<sub>i</sub> V<sub>i</sub>** contribute to the actual data and the rest can be discarded without affecting the information in the data. In our case, we choose to work with the first two singular values. Fig.S4b represents the first two columns of **V**, the blue trace is **σ<sub>1</sub> V<sub>1</sub>** and shows the fluorescence depletion spectrum as a function of frequency. The dotted lines show **σ<sub>2</sub> V<sub>2</sub>** which represents the change in the shape of the spectrum - the spectrum shifts to lower frequencies. The orange line is the time dependence of the frequency shift in the spectrum and that is given by plotting **σ<sub>2</sub> U<sub>2</sub>**. We fit this using an exponential function of the form **y = y<sub>0</sub> e<sup>-kt</sup>**. The decay constant (**k**) gives the rate of formation of SiOH<sup>+</sup>.

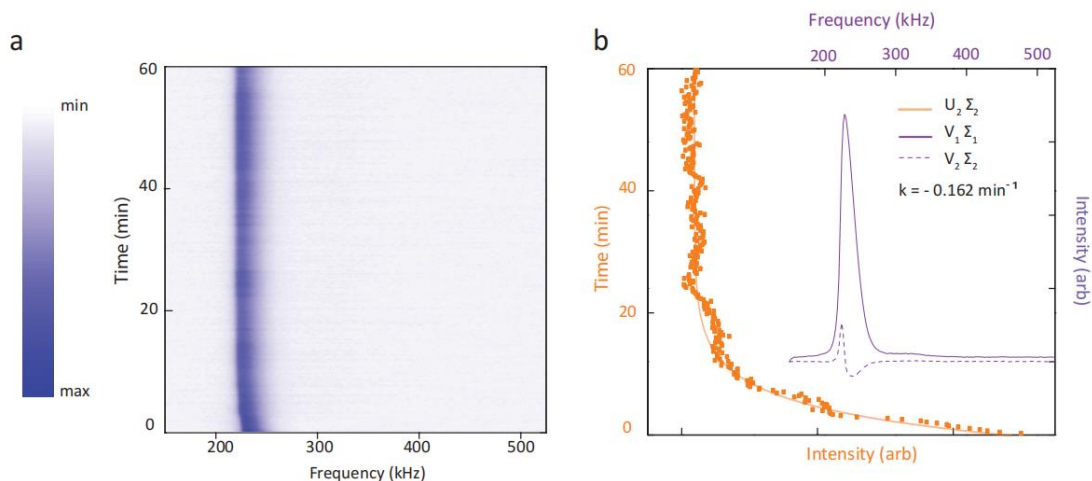

**Fig. S4 a:** Experimental data showing the fluorescence of  $\text{Ba}^+$  as a function of the RF chirp frequency and time. **b:** Selected components from the singular value decomposition of the data set shown in **a**.

SVD can separate out several components of the data such as the mass spectrum, change in the mass spectrum with time and the broadening of the mass spectrum (described by  $\mathbf{U}_1 \sigma_1$ ,  $\mathbf{U}_2 \sigma_2$ , and  $\mathbf{U}_3 \sigma_3$  respectively; these vectors are also orthogonal to each other). We then fit only the change in the peak as a function of time to an exponential decay, (neglecting amplitude fluctuations in the fluorescence and broadening effects). Since we already know that there is a linear dependency between the change in the center of the peak and the fraction of  $\text{SiO}^+$  in the system, the fit for the change in the center of the peak also gives us the rate of the reaction.

## V. Potential Energy Surface

Similar to our previous work on ion-molecule reactions,<sup>4,5</sup> the global potential energy surface (PES) of  $\text{SiOH}_2^+(\text{X}^2\text{A})$  consists of an analytical long-range interaction term and fitted PES from *ab initio* points in the short range. The long-range (LR) term in the  $\text{SiO}^+ + \text{H}_2$  reactant channel asymptote, which is important for an accurate description of the reaction kinetics at low temperatures, includes the leading electrostatic interactions between the two reactants

when they are far apart. On the other hand, the fitted PES describes all other regions where chemical interaction dominates. These two segments are connected smoothly via a switching function, as discussed below.

#### a. Long-range part of the PES

In describing the long-range interaction, the ion  $\text{SiO}^+$  is approximated as a point charge, and  $q$  denotes the charge of the molecular ion (+1).  $\text{H}_2$  is a homonuclear diatomic molecule without a dipole moment. Its parallel and perpendicular components of the polarizability are  $\alpha_{||}=0.4793 \text{ \AA}^3$  and  $\alpha_{\perp}=0.1653 \text{ \AA}^3$ , and its overall polarizability can be approximated as  $\alpha = \alpha_{||} + 2\alpha_{\perp}=0.81 \text{ \AA}^3$ . It also has a quadrupole moment ( $\theta=0.63 \text{ esu}$ ).<sup>6</sup> The long-range interaction between the ion  $\text{SiO}^+$  and molecule  $\text{H}_2$  is dominated by the leading electrostatic terms, which is proportional to the inverse powers of the distance  $R$  between the two moieties. Specifically, the electrostatic potential  $V_{\text{ES}}$  includes charge-quadrupole,  $V_{q-\theta}(\xi, \theta)$ , and charge-induced dipole,  $V_{q-\alpha}(\xi, \theta)$ , interactions:<sup>7</sup>

$$V_{\text{ES}} = V_{q-\theta} + V_{q-\alpha} = \frac{1}{2}q\theta\xi^{-3}(3\cos^2\theta - 1) - \frac{1}{2}q^2\xi^{-4}[\alpha + \frac{\alpha_{||}+\alpha_{\perp}}{3}(3\cos^2\theta - 1)] \quad (\text{ii})$$

where  $\xi$  is the separation between the center of charge of the  $\text{SiO}^+$  ion and the center of mass of the hydrogen molecule, and  $\theta$  is the angle between  $\xi$  and the H-H internuclear bond vector. The center of charge is defined as  $\vec{c}_{\text{SiO}^+} = (\sum_i q_i \vec{c}_i) / (\sum_i q_i)$  in analogy to the center of mass, where  $\vec{c}_i$  are the atomic coordinates and the atomic charges  $q_i$  were calculated using the electrostatic potential on a grid (CHelpG) point selection algorithm.<sup>8</sup>

The LR PES can be written as:

$$V_{\text{LR}} = V_{\text{SiO}^+} + V_{\text{H}_2} + V_{\text{ES}} \quad (\text{iii})$$

where  $V_{\text{SiO}^+}$  and  $V_{\text{H}_2}$  are the potential energy curves (PECs) for the isolated  $\text{SiO}^+$  and  $\text{H}_2$  molecules, which were spline-interpolated from *ab initio* data points at the level of UCCSD(T)-F12b (unrestricted coupled cluster singles, doubles and perturbative triples)<sup>9</sup> with the correlation-consistent polarized core-valence quadruple-zeta basis set for explicitly correlated wavefunctions (cc-pCVQZ-F12).<sup>10</sup> The explicit treatment of the electron-electron interaction (F12) allows a fast convergence with respect to the complete basis set limit.<sup>11</sup> All the potential energies are related to the potential minimum with the  $\text{SiO}^+-\text{H}_2$  separation of 100.0  $\text{\AA}$ .

It should be noted that the adiabatic potential  $V_{\text{SiO}^+}$  is the lower adiabat of the  $X^2\Sigma^+$  and  $A^2\Pi$  states of  $\text{SiO}^+$  (as shown in Fig. S5). Since the  $\text{SiO}^+$  species in the  $\text{SiO}^+ + \text{H}_2 \rightarrow \text{SiOH}^+ + \text{H}$  reaction is always in the lowest vibrational level under experimental conditions, it is safe to assume that the reaction is well described on the adiabatic ground state PES of  $\text{SiOH}_2^+$  in the reactant asymptote. However, it is conceivable that the A state might be involved in the strongly interacting region, particularly when  $\text{SiO}^+$  is in a super rotor state. The neglect of non-adiabatic effects here is one of the possible reasons for the quantitative discrepancy of the calculated results from the experiment at high rotational states.

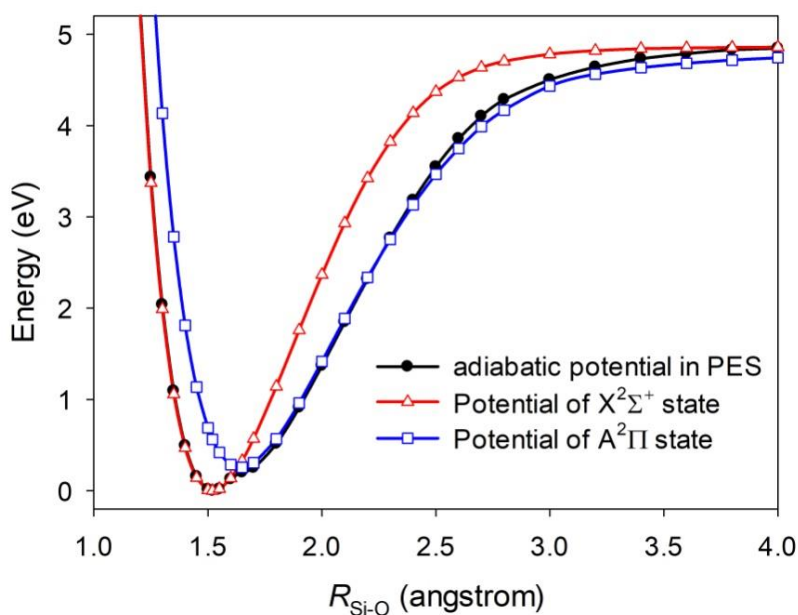

**Fig. S5:** The potential energy curves of  $\text{SiO}^+$

#### b. Fitted PES

For the short-range PES, *ab initio* calculations were carried out at the level of UCCSD(T)-F12b/cc-pCVQZ-F12, the same as the PEC calculations of  $\text{SiO}^+$  and  $\text{H}_2$ . All *ab initio* calculations were performed with MOLPRO.<sup>12</sup> The stationary points along the reaction path, along with their geometries, relative energies and harmonic frequencies are listed in Tables S1 and S2.

To generate the *ab initio* points for fitting the PES, grids of points in the appropriate coordinates along the reaction pathway were first calculated in various regions. In total, 20147 points were fit using the high-fidelity permutation invariant polynomial-neural network (PIP-NN) method.<sup>13</sup> In particular, 17 PIPs up to second order have included as the

input layer of the NN in order to take advantage of the permutation symmetry of this ABC<sub>2</sub> system. Morse-like variables,  $p_{ij} = \exp(-r_{ij}/a)$ , were used to construct the PIPs with  $a = 2.0$  Å as the length parameter, in which  $r_{ij}$  denotes the internuclear distance between the  $i^{\text{th}}$  and  $j^{\text{th}}$  atoms. The NN consists of 2 hidden layers, each with 30 and 60 interconnected neurons. The total number of parameters is thus 2460. In each NN fitting, the data were divided randomly into three sets, namely the training (90% of the data points), validation (5%), and test (5%) sets. The early stop method was used to avoid overfitting.<sup>14</sup> The final PIP-NN PES was chosen as the average of three best fits, as suggested by the NN ensemble approach to minimize random errors.<sup>15</sup> The RMSEs for the training/validation/test sets of the three best fits are 16.5/16.9/20.4, 17.3/18.2/21.2, and 17.7/18.2/21.2 meV, respectively. The overall RMSE of the PES is 16.4 meV. The geometries and energies of the stationary points on the PES is compared in Tables S1 and S2. The agreement with the values determined directly from *ab initio* calculations is quite satisfactory.

The overall PES is switched smoothly from the long-range PES to the fitted PES:

$$V = SV_{\text{fit}} + (1 - S)V_{\text{LR}} \quad (\text{iv})$$

where the switching function is defined:

$$S = \frac{1 - \tanh(3(R - 7.0))}{2} \quad (\text{v})$$

where  $R$  is the distance between the center of mass of the two reactants. As a result, the overall PES is dominated by  $V_{\text{LR}}$  for  $R > 7.5$  Å, while by  $V_{\text{fit}}$   $R < 6.5$  Å.

**Table S1:** Energies and geometries in internal coordinates of the stationary points on the PES for the  $\text{SiO}^+ + \text{H}_2 \rightarrow \text{SiOH}^+ + \text{H} / \text{Si}^+ + \text{H}_2\text{O}$  reaction.

| Species                                                                                                                                                                        |                  | $\Delta E$ (eV) | $r_{\text{SiO}}$ (Å) | $r_{\text{HH}}$ (Å) | $r_{\text{OH}}/r_{\text{SiH}}$ (Å) | $\vartheta_{\text{SiOH}}/\vartheta_{\text{OSiH}}$ (°) | $\phi_{\text{SiOH}}$ (°) |
|--------------------------------------------------------------------------------------------------------------------------------------------------------------------------------|------------------|-----------------|----------------------|---------------------|------------------------------------|-------------------------------------------------------|--------------------------|
| $\text{SiO}^+ + \text{H}_2$                                                                                                                                                    | <i>ab initio</i> | 0.0             | 1.63                 | 0.74                |                                    |                                                       |                          |
|                                                                                                                                                                                | PES              | 0.0             | 1.62                 | 0.74                |                                    |                                                       |                          |
| $\text{SiOH}^+ + \text{H}$                                                                                                                                                     | <i>ab initio</i> | -1.76           | 1.54                 |                     | 0.96/2.50                          | 180.0/0.0                                             |                          |
|                                                                                                                                                                                | PES              | -1.76           | 1.54                 |                     | 0.96/2.50                          | 180.0/0.0                                             |                          |
| $\text{Si}^+ + \text{H}_2\text{O}$                                                                                                                                             | <i>ab initio</i> | -0.50           |                      | 1.52                | 0.96/-                             |                                                       |                          |
|                                                                                                                                                                                | PES              | -0.50           |                      | 1.51                | 0.96/-                             |                                                       |                          |
| 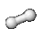<br>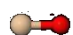 IM1 | <i>ab initio</i> | -0.33           | 1.53                 | 0.77                | 2.87/2.11                          | 44.3/115.9                                            | 0.0                      |
|                                                                                                                                                                                | PES              | -0.31           | 1.51                 | 0.76                | 2.81/2.10                          | 49.9/118.5                                            | 0.0                      |

|                                                                                         |                  |       |      |      |            |             |       |
|-----------------------------------------------------------------------------------------|------------------|-------|------|------|------------|-------------|-------|
| 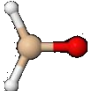 IM2   | <i>ab initio</i> | -1.11 | 1.61 | 2.66 | 1.46/2.58  | 31.2/114.3  | 0.0   |
|                                                                                         | PES              | -1.12 | 1.61 | 2.66 | 1.47 /2.59 | 30.8/115.1  | 0.0   |
| 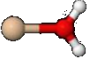 IM3   | <i>ab initio</i> | -2.61 | 1.87 | 1.59 | 0.97/-     | 124.8/18.2  | 180.0 |
|                                                                                         | PES              | -2.60 | 1.84 | 1.60 | 0.97/-     | 123.3/17.9  | 180.0 |
| 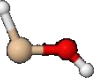 IM4   | <i>ab initio</i> | -3.01 | 1.57 | 3.48 | 0.96/1.49  | 133.2/111.9 | 0.0   |
|                                                                                         | PES              | -3.02 | 1.58 | 3.48 | 0.97/1.50  | 133.1/111.9 | 0.0   |
| 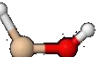 IM5   | <i>ab initio</i> | -2.92 | 1.56 | 3.10 | 0.96/1.50  | 138.3/120.2 | 180.0 |
|                                                                                         | PES              | -2.92 | 1.58 | 3.16 | 0.97/1.51  | 135.3/120.8 | 180.0 |
| 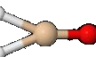 TS0*  | <i>ab initio</i> | —     | —    | —    | —          | —           | —     |
|                                                                                         | PES              | 1.58  | 1.53 | 1.33 | -/1.74     | 11.9/157.6  | 0.0   |
| 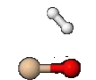 TS1   | <i>ab initio</i> | -0.11 | 1.61 | 0.81 | 1.60/2.37  | 84.7/76.2   | 0.0   |
|                                                                                         | PES              | -0.12 | 1.61 | 0.81 | 1.60/2.36  | 84.8/67.4   | 0.0   |
| 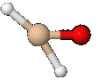 TS2   | <i>ab initio</i> | -0.14 | 1.56 | 3.01 | 1.54/1.57  | 61.0/58.5   | 0.0   |
|                                                                                         | PES              | -0.15 | 1.56 | 3.01 | 1.53/1.57  | 60.9/58.6   | 0.0   |
| 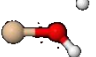 TS3 | <i>ab initio</i> | -0.69 | 1.63 | 1.84 | 1.46/2.39  | 131.6/22.8  | 180.0 |
|                                                                                         | PES              | -0.68 | 1.63 | 1.84 | 1.45/2.38  | 132.5/22.3  | 180.0 |
| 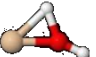 TS4 | <i>ab initio</i> | -1.07 | 1.69 | 2.08 | 1.27/1.74  | 70.1/43.5   | 180.0 |
|                                                                                         | PES              | -1.04 | 1.68 | 2.11 | 1.24/1.72  | 70.1/42.8   | 180.0 |
| 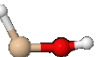 TS5 | <i>ab initio</i> | -2.89 | 1.54 | 3.39 | 0.96/1.51  | 170.5/117.5 | 180.0 |
|                                                                                         | PES              | -2.69 | 1.53 | 3.42 | 0.96/1.51  | 172.3/118.6 | 180.0 |

\* TS0 is not optimized by UCCSD(T)-F12 method.

**Table S2.** Harmonic frequencies of the stationary points on the PES for the  $\text{SiO}^+ + \text{H}_2 \rightarrow \text{SiOH}^+ + \text{H} / \text{Si}^+ + \text{H}_2\text{O}$  reaction

| Species                            |                  | Frequency (cm <sup>-1</sup> ) |        |        |        |        |        |
|------------------------------------|------------------|-------------------------------|--------|--------|--------|--------|--------|
|                                    |                  | 1                             | 2      | 3      | 4      | 5      | 6      |
| SiO <sup>+</sup> + H <sub>2</sub>  | <i>ab initio</i> | 1150.7                        | 4403.7 |        |        |        |        |
|                                    | PES              | 1145.8                        | 4401.0 |        |        |        |        |
| SiOH <sup>+</sup> + H              | <i>ab initio</i> | 354.1                         | 1145.3 | 3846.1 |        |        |        |
|                                    | PES              | 353.4                         | 1143.8 | 3842.6 |        |        |        |
| Si <sup>+</sup> + H <sub>2</sub> O | <i>ab initio</i> | 1649.5                        | 3835.0 | 3945.6 |        |        |        |
|                                    | PES              | 1649.4                        | 3831.9 | 3942.1 |        |        |        |
| IM1                                | <i>ab initio</i> | 217.6                         | 304.4  | 535.5  | 747.9  | 989.7  | 3970.4 |
|                                    | PES              | 246.7                         | 263.5  | 490.2  | 714.2  | 1196.5 | 4006.1 |
| IM2                                | <i>ab initio</i> | 506.1                         | 683.8  | 841.2  | 1002.2 | 2282.5 | 2357.1 |
|                                    | PES              | 499.1                         | 676.7  | 838.3  | 985.8  | 2287.7 | 2365.8 |

|     |                  |       |       |        |        |        |         |
|-----|------------------|-------|-------|--------|--------|--------|---------|
| IM3 | <i>ab initio</i> | 402.1 | 487.9 | 665.8  | 1654.3 | 3678.4 | 3770.9  |
|     | PES              | 465.0 | 496.0 | 661.2  | 1655.0 | 3551.2 | 3794.7  |
| IM4 | <i>ab initio</i> | 540.4 | 593.9 | 720.0  | 1079.0 | 2084.4 | 3812.8  |
|     | PES              | 539.0 | 587.4 | 720.1  | 1083.3 | 2100.8 | 3839.7  |
| IM5 | <i>ab initio</i> | 441.3 | 447.7 | 696.9  | 1113.8 | 2037.7 | 3812.2  |
|     | PES              | 440.6 | 450.6 | 695.7  | 1112.3 | 2034.6 | 3808.5  |
| TS0 | <i>ab initio</i> | -     | -     | -      | -      | -      | -       |
|     | PES              | 266.3 | 649.7 | 1440.3 | 1820.2 | 335.9i | 1828.0i |
| TS1 | <i>ab initio</i> | 350.7 | 405.8 | 701.6  | 939.1  | 3212.8 | 464.6i  |
|     | PES              | 350.9 | 418.2 | 699.4  | 964.4  | 3117.9 | 476.4i  |
| TS2 | <i>ab initio</i> | 454.1 | 587.2 | 1072.4 | 1945.0 | 2219.3 | 1437.1i |
|     | PES              | 473.1 | 605.7 | 1067.6 | 1959.6 | 2201.7 | 1428.2i |
| TS3 | <i>ab initio</i> | 359.0 | 596.8 | 908.8  | 1077.2 | 3747.8 | 2845.7i |
|     | PES              | 408.7 | 593.7 | 906.8  | 1076.1 | 3744.9 | 2831.8i |
| TS4 | <i>ab initio</i> | 699.9 | 880.1 | 1693.0 | 3610.9 | 119.8i | 1712.3i |
|     | PES              | 826.1 | 928.0 | 1944.0 | 3617.9 | 323.8i | 1764.6i |
| TS5 | <i>ab initio</i> | 268.8 | 689.4 | 1154.1 | 1997.8 | 3885.0 | 373.7i  |
|     | PES              | 269.9 | 687.7 | 1152.6 | 1993.7 | 3881.7 | 374.1i  |

- 1 Rosner, S. D., Cameron, R., Scholl, T. J. & Holt, R. A. A study of the  $X^2\Sigma^+$  and  $A^2\Pi$  States of  $\text{SiO}^+$  using fast-ion-beam laser spectroscopy. *J. Mol. Spectrosc.* **189**, 83-94 (1998).
- 2 Antonov, I. O. *et al.* Precisely spun super rotors. *Nat. Commun.* **12**, 2201 (2021).
- 3 Qin, Z., Bai, T., Zhao, J. & Liu, L. Transition properties between low-lying electronic states of  $\text{SiO}^+$ . *J. Mol. Spectrosc.* **370**, 111298 (2020).
- 4 Li, A. & Guo, H. A full-dimensional global potential energy surface of  $\text{H}_3\text{O}^+(\tilde{a}^3A)$  for the  $\text{OH}^+(\tilde{X}^3\Sigma^-) + \text{H}_2(\tilde{X}^1\Sigma_g^+) \rightarrow \text{H}(^2S) + \text{H}_2\text{O}^+(\tilde{X}^2B_1)$  reaction. *J. Phys. Chem. A* **118**, 11168-11176 (2014).
- 5 Shi, W., Jia, T. & Li, A. Quasi-classical trajectory analysis with isometric feature mapping and locally linear embedding: deep insights into the multichannel reaction on an  $\text{NH}_3^+(^4A)$  potential energy surface. *Phys. Chem. Chem. Phys.* **22**, 17460-17471 (2020).
- 6 Simonyan, V. V., Diep, P. & Johnson, J. K. Molecular simulation of hydrogen adsorption in charged single-walled carbon nanotubes. *J. Chem. Phys.* **111**, 9778-9783 (1999).
- 7 Buckingham, A. D. Permanent and induced molecular moments and long-range intermolecular forces in *Advances in Chemical Physics* 107-142 (John Wiley & Sons, Inc., 2007).
- 8 Breneman, C. M. & Wiberg, K. B. Determining atom-centered monopoles from molecular electrostatic potentials - the need for high sampling density in formamide conformational-analysis. *J. Comput. Chem.* **11**, 361-373 (1990).
- 9 Knizia, G., Adler, T. B. & Werner, H.-J. Simplified CCSD(T)-F12 methods: theory and benchmarks. *J. Chem. Phys.* **130**, 054104 (2009).
- 10 Pritchard, B. P., Altarawy, D., Didier, B., Gibson, T. D. & Windus, T. L. New basis set exchange: An open, up-to-date resource for the molecular sciences community. *J. Chem. Inf. Model.* **59**, 4814-4820 (2019).

- 11 Feller, D. & Peterson, K. A. An expanded calibration study of the explicitly correlated CCSD(T)-F12b method using large basis set standard CCSD(T) atomization energies. *J. Chem. Phys.* **139**, 084110 (2013).
- 12 Werner, H. J., Knowles, P. J., Knizia, G., Manby, F. R. & Schütz, M. Molpro: a general-purpose quantum chemistry program package. *WIREs Comput. Mol. Sci.* **2**, 242-253 (2012).
- 13 Jiang, B., Li, J. & Guo, H. Potential energy surfaces from high fidelity fitting of ab initio points: The permutation invariant polynomial-neural network approach. *Int. Rev. Phys. Chem.* **35**, 479 (2016).
- 14 Raff, L. M., Komanduri, R., Hagan, M. & Bukkapatnam, S. T. S. *Neural Networks in Chemical Reaction Dynamics*. (Oxford University Press, 2012).
- 15 Zhou, Z.-H., Wu, J. & Tang, W. Ensembling neural networks: Many could be better than all. *Art. Intel.* **137**, 239-263 (2002).
